# Supplementary material for: Differentiable and Scalable Generative Adversarial Models for Data Imputation
Source: arXiv:2201.03202 source file (2022-01-10)
Supplement: Supplementary file 1 [file 8.appendix.tex]

\section{Appendix for Detailed Proofs}
\label{sec:appendix-proof}
\setcounter{table}{0}
\setcounter{equation}{0}
\setcounter{proposition}{0}
\setcounter{theorem}{0}
\newenvironment{proof}{\textit{Proof}.}{\hfill$\square$}

\subsection{Proof of Proposition 1}
\label{app:pro1}
\begin{proposition}
The MS divergence gradient function $g(\theta)$ can be calculated by
\begin{equation}
\begin{aligned} \nonumber
    g(\theta)&=\frac{1}{2n}\nabla_{\theta}\mathcal{S}_{\mathbf{m}}(\bar{\mathbf{X}}\odot\mathbf{M}, \mathbf{X} \odot \mathbf{M})\\
  &=\left[\frac{1}{2n}\nabla_{\bar{\mathbf{X}}}\mathcal{S}_{\mathbf{m}}(\bar{\mathbf{X}}\odot\mathbf{M}, \mathbf{X} \odot \mathbf{M})\right]^{\top}\nabla_{\theta}\bar{\mathbf{X}}\\%\mathcal{M}(\theta)\\
    &=\frac{1}{n}\sum_{j=1}^{n} \big[\sum_{i=1}^{n}\mathbf{P}^{\star}_{ij}\cdot (\bar{\mathbf{\mathbf{x}}}_{i} \odot \mathbf{m}_{i} - {\mathbf{x}}_{j}\odot\mathbf{m}_{j}) \cdot \mathcal{T}(\mathbf{m}_{i}) \cdot \nabla_{\theta} \bar{\mathbf{x}}_{i} \big], %\nabla_{\theta}\mathcal{M}(\theta)
\label{eq:paramchange-app}
\end{aligned}
\end{equation}
where $\nabla_{\theta}\mathcal{S}_{\mathbf{m}}(\cdot)$ and $\nabla_{\bar{\mathbf{X}}}\mathcal{S}_{\mathbf{m}}(\cdot)$ is the derivative of $\mathcal{S}_{\mathbf{m}}(\cdot)$ with respect to the model parameters $\theta$ and the reconstructed matrix $\bar{\mathbf{X}}$, respectively.
$\nabla_{\theta}\bar{\mathbf{X}}$ is the derivative of $\bar{\mathbf{X}}$ with respect to $\theta$.
$\mathbf{P}^{\star}$ is the optimal (regularized) transport plan.
$\mathcal{T}(\mathbf{m}_{i})$ is to transform a mask vector $\mathbf{m}_{i}$ to a diagonal matrix.
\end{proposition}

\begin{proof}
First of all, by the barycentric transport map \cite{cuturi2014fast}, we obtain that $\forall k \in {1,\dots,N}$,
\begin{align*}
    \nabla{\bar{\mathbf{x}}_{k}}OT_{\lambda}(\mathbf{M} \odot \bar{\mathbf{X}},\mathbf{M} \odot {\mathbf{X}}) = \sum_{j=1}^{n}\mathbf{P}^{\star}_{kj} \cdot(\mathbf{m}_{k} \odot \bar{\mathbf{x}}_{k} - \mathbf{m}_{j} \odot \mathbf{x}_{j}). %\cdot \mathcal{T}(\mathbf{m_i})
\end{align*}
Then, by the chain rule, we can infer that the gradient of $\mathcal{I}(\theta)$ is
\begin{align*}
    \nabla_{\theta}\mathcal{I}(\theta)&=
    [\frac{1}{2n}\nabla_{\bar{\mathbf{X}}}\mathcal{S}_{}(\mathbf{M} \odot \bar{\mathbf{X}}_{},\mathbf{M} \odot {\mathbf{X}}_{})]^{\top}\nabla_{\theta}\bar{\mathbf{X}}\\
    &=\frac{1}{N}\sum_{i=1}^{n}\bigg[\sum_{j=1}^{n}\mathbf{P}^{\star}_{ij}\cdot(\mathbf{m}_{i} \odot \bar{\mathbf{x}}_{i} - \mathbf{m}_{j} \odot {\mathbf{x}}_{j})\bigg]\cdot \mathcal{T}(\mathbf{m}_i) \cdot \nabla_{\theta}\bar{\mathbf{x}}_{i}\\
    &=\frac{1}{n}\sum_{j=1}^{n}\bigg[\sum_{i=1}^{n}\mathbf{P}^{\star}_{ij}\cdot(\mathbf{m}_{i} \odot \bar{\mathbf{x}}_{i} - \mathbf{m}_{j} \odot {\mathbf{x}}_{j})\cdot {\mathcal{T}}(\mathbf{m}_i) \cdot \nabla_{\theta}\bar{\mathbf{x}}_{i}\bigg].
\end{align*}
\end{proof}

\subsection{Proof of Theorem 1}
\label{app:theo1}

\begin{theorem}
Given the parameter $\theta_0$ of $\mathcal{M}_0$ with the size-$n_0$ samples, the {\color{blue}conditional  distribution of $\hat{\theta}_n$ in $\mathcal{M}_n$ with a size-$n$ sample set satisfies}
\begin{equation}\nonumber
    \hat{\theta}_n|\theta_{0} \to \mathcal{N}(\theta_{0}, \eta \mathbf{H}^{-1}),  \quad \text{with}\quad \eta \asymp e^{\frac{6}{\lambda}}(1 + \frac{1}{\lambda^{\lfloor d/2 \rfloor}})^{2} \cdot \left(\frac{1}{n_0} - \frac{1}{n}\right)
\end{equation}
as $n_0 \to \infty$ and $n \to \infty$, where
$\lambda$ is a hyper-parameter in the MS divergence. % and $\eta \asymp \frac{e^{\frac{6}{\lambda}}}{\lambda^{2\lfloor d/2 \rfloor}} \cdot \left(\frac{1}{n_0} - \frac{1}{n}\right)$ means that
$\mathcal{N}(\theta_{0}, \eta \mathbf{H}^{-1})$ denotes a multivariate normal distribution with mean $\theta_{0}$ and covariance matrix $\eta \mathbf{H}^{-1}$.
$\mathbf{H}$ is the Hessian matrix of the MS divergence imputation loss function with the given parameter $\theta_{0}$.
\end{theorem}
\begin{proof}
First, we can derive the distribution of $\hat{\theta}_{0} - \theta_{\infty}$ by the multivariate central limit theorem.
$\theta_{\infty}$ is the conceptual optimal parameters when the training sample size approaches infinity.
Then we can derive the distribution of $\hat{\theta}_{0} - \hat{\theta}_{n}$ since $\hat{\theta}_{0} - \hat{\theta}_{n} = (\hat{\theta}_{0} - \theta_{\infty}) - (\hat{\theta}_{n} - \theta_{\infty})$.
Finally, we can exploit the Bayes theorem to infer the distribution of $\hat{\theta}_{n}|\theta_{0}$ from the distribution of $\hat{\theta}_{0} - \hat{\theta}_{n}$.

Since $\hat{\theta}_{0}$ is obtained by finding the parameter at which $g(\theta)$ becomes zero, it satisfies $g(\theta_{0}) = 0$.
According to the mean-value theorem, there exists $\bar{\theta}_{0}$ between $\theta_{0}$ and $\theta_{\infty}$ that satisfies:
\begin{equation} \nonumber
    g'(\bar{\theta}_{0})(\theta_{0} - \theta_{\infty}) = g(\theta_{0}) - g(\theta_{\infty}) = -g(\theta_{\infty}),
\end{equation}
%where $H(\bar{\theta})$ is the Hessian of $f_{n}(\theta)$ evaluted at $\bar{\theta}$.
Note that $\theta_{0}$ is simply an instance from the distribution $\hat{\theta}_{0}$. Furthermore, we have
\begin{align} \nonumber
    (\hat{\theta}_{0} - \theta_{\infty}) =& - g'(\theta_{\infty})^{-1}\cdot g(\theta_{\infty}) \\ \label{eq:second}
     = &-  g'(\theta_{\infty})^{-1}\cdot (\sum_{j=1}^{n_0}\left[\sum_{i=1}^{n_0}\mathbf{P}^{\star}_{ij}\cdot (\mathbf{m}_{i} \odot \bar{\mathbf{\mathbf{x}}}_{i} - \mathbf{m}_{j} \odot {\mathbf{x}}_{j}) \cdot \mathcal{T}(\mathbf{m_{i}}) \cdot \nabla_{\theta_{\infty}} \bar{\mathbf{x}}_{i} \right])\\ \label{eq:clt}
    & \xrightarrow{n_0 \to \infty} \mathcal{N}(0, \zeta(\lambda, n_{0})\mathbf{H}^{-1}\mathbf{J}\mathbf{H}^{-1}) \\\label{eq:info} \nonumber
     = &\mathcal{N}(0, \zeta(\lambda)\frac{1}{n_{0}}\mathbf{H}^{-1}),
\end{align}
%\frac{e^{\frac{\kappa}{\lambda}}}{{\lambda^{\lfloor d/2 \rfloor}\sqrt{n_0}}} \cdot
where $\zeta(\lambda) \asymp {e^{\frac{2\kappa}{\lambda}}}(1+\frac{1}{\lambda^{\lfloor d/2 \rfloor}})^{2}$, $\mathbf{J}$ is the information matrix and $\mathbf{H}$ is the Hessian matrix of the MS estimator.
The transition from Eq.$\ref{eq:second}$ to Eq.$\ref{eq:clt}$ is based on the multidimensional central limit theorem and the fact that the simple complexity for Sinkhorn divergence is $O(\frac{e^{\frac{\kappa}{\lambda}}}{\sqrt{n}}(1+\frac{1}{\lambda^{\lfloor d/2 \rfloor}}))$, where $\kappa = 2L|\mathcal{X}|+ \vert|f_c\vert|_{\infty}$. Here, $|\mathcal{X}|$ is the diameter
%$\rm{sup}\{\vert|\mathbf{x} - \mathbf{x'}\vert| | \mathbf{x}, \mathbf{x'} \in \mathcal{X}\}$
$\rm{sup}\{\lVert \mathbf{x} - \mathbf{x'}\rVert | \mathbf{x}, \mathbf{x'} \in \mathcal{X}\}$
of $\mathcal{X}$ and $L$ is the Lipschitz constant for the cost function $f_c$.
In our case,  $|\mathcal{X}|$ and $L$ will both be 1, since the input data will be normalized to $[0,1]^{d}$ and the cost function $f_c$ is a two norm function. Moreover, the information  matrix inequality that $\mathbf{J} = - \mathbf{H}$ implies the last equation.

%Now, we derive the distribution of $\hat{\theta}_{n} - \hat{\theta}_{N}$.
Then, we can derive the distribution of $\hat{\theta}_{0} - \hat{\theta}_{n}$ since $\hat{\theta}_{0} - \hat{\theta}_{n} = (\hat{\theta}_{0} - \theta_{\infty}) - (\hat{\theta}_{n} - \theta_{\infty})$.
By exploiting the fact that $\mathbf{X}_{n}$ can be regarded as a union of $\mathbf{X}_{0}$ and $\mathbf{X}_{n} - \mathbf{X}_{0}$, we introduce two random variables $V_1$, $V_2$ independently following $\mathcal{N}(0,  \zeta(\lambda)\mathbf{H}^{-1})$ to separately capture the randomness stemming from $\mathbf{X}_{0}$ and $\mathbf{X}_{n} - \mathbf{X}_{0}$.
From Eq. \ref{eq:clt}, $\hat{\theta}_{0} - \theta_{\infty}$ $\rightarrow$ $\frac{1}{\sqrt{n_0}}V_{1}$. then,
\begin{align}
    &\hat{\theta}_{0} - \hat{\theta}_{n} = (\hat{\theta}_{0} - \theta_{\infty}) - (\hat{\theta}_{n} - \theta_{\infty})\\  \nonumber
    &=-\frac{1}{\sqrt{n_0}}g'(\bar{\theta}_{0})^{-1}(\frac{1}{\sqrt{n_0}} \sum_{j=1}^{n_0} \big[\sum_{i=1}^{n_0}\mathbf{P}^{\star}_{ij}\cdot(\mathbf{m}_{i} \odot \bar{\mathbf{\mathbf{x}}}_{i} - \mathbf{m}_{j} \odot {\mathbf{x}}_{j}) \cdot \mathcal{T}(\mathbf{m}_{i}) \cdot \nabla_{\theta} \bar{\mathbf{x}}_{i} \big])\\ \nonumber
    &+ \frac{1}{\sqrt{n}}g'(\bar{\theta}_{n})^{-1}(\frac{\sqrt{n_0}}{\sqrt{n}}\frac{1}{\sqrt{n_0}}\sum_{j=1}^{n_0} \big[\sum_{i=1}^{n}\mathbf{P}^{\star}_{ij}\cdot(\mathbf{m}_{i} \odot \bar{\mathbf{\mathbf{x}}}_{i} - \mathbf{m}_{j} \odot {\mathbf{x}}_{j}) \cdot \mathcal{T}(\mathbf{m}_{i}) \cdot \nabla_{\theta} \bar{\mathbf{x}}_{i} \big]\\ \nonumber
    &+ \frac{\sqrt{n-n_0}}{\sqrt{n}} \frac{1}{\sqrt{n - n_0}} \sum_{j=n_0+1}^{n} \big[\sum_{i=1}^{n}\mathbf{P}^{\star}_{ij}\cdot(\mathbf{m}_{i} \odot \bar{\mathbf{\mathbf{x}}}_{i} - \mathbf{m}_{j} \odot {\mathbf{x}}_{j}) \cdot \mathcal{T}(\mathbf{m}_{i}) \cdot \nabla_{\theta} \bar{\mathbf{x}}_{i} \big]) \\
    &\xrightarrow{n_0 \to \infty \text{ and }  n \to \infty} (\frac{1}{\sqrt{n_0}} - \frac{\sqrt{n_0}}{n})V_{1} - \frac{\sqrt{n - n_0}}{\sqrt{n}}V_{2} \label{comb1} \\
    & \sim \mathcal{N}(0, (\frac{1}{n_0} - \frac{1}{n})\cdot \zeta(\lambda) \cdot \mathbf{H}^{-1}),\label{comb2}
\end{align}
where $\bar{\theta}_{0}$ is between $\theta_{0}$ and $\theta_{\infty}$ and $\bar{\theta}_{n}$ is between $\theta_{n}$ and $\theta_{\infty}$.
To get the transition from Eq. $\ref{comb1}$ to Eq. $\ref{comb2}$, we exploit the fact that $\hat{\theta}_{0} - \hat{\theta}_{n}$ asymptotically follows a normal distribution, which is linearly composed of two random variables independently following normal distributions.

Finally, we infer the core of Theorem 1, i.e., the conditional parameter distribution $\hat{\theta}_{n}|\theta_{0}$.
Observe that $\hat{\theta}_{0} - \hat{\theta}_{n}$ and $\hat{\theta}_{n} - \theta_{\infty}$ are independent because they are jointly normally distributed and the covariance between them is zero, as shown below:
\begin{equation}
    \begin{aligned}\nonumber
    &Cov(\hat{\theta}_{0} - \hat{\theta}_{n}, \hat{\theta}_{n} - \theta_{\infty})\\
    &= \frac{1}{2}(Var(\hat{\theta}_{0} - \hat{\theta}_{n} + \hat{\theta}_{n} - \theta_{\infty}) - Var(\hat{\theta}_{0} - \hat{\theta}_{n}) - Var(\hat{\theta}_{n} - \theta_{\infty}))\\
    &= \frac{1}{2} (\frac{1}{n_0} - (\frac{1}{n_0} - \frac{1}{n}) - \frac{1}{n})\cdot \zeta(\lambda) \cdot\mathbf{H}^{-1} = 0.
    \end{aligned}
\end{equation}
Thus, Var($\hat{\theta}_{0} - \hat{\theta}_{n}$) = Var($\hat{\theta}_{0} - \hat{\theta}_{n}|\theta_{n}$) = $\eta \mathbf{H}^{-1}$, which implies
\begin{equation}
\label{condistri}
    \hat{\theta}_{0} \sim (\theta_{n}, \eta \mathbf{H}^{-1}), \quad \eta \asymp e^{\frac{6}{\lambda}}(1 + \frac{1}{\lambda^{\lfloor d/2 \rfloor}})^{2} \cdot \left(\frac{1}{n_0} - \frac{1}{n}\right)
\end{equation}
Using Bayes' theorem,
\begin{equation} \nonumber
    \mathbb{P}(\theta_{n}|\theta_{0}) = (1/Z)\mathbb{P}(\theta_{0}|\theta_{n})\mathbb{P}(\theta_{n}),
\end{equation}
for some normalization constant $Z$. Since there is no preference on $\mathbb{P}(\theta_{n})$, we set a constant to $\mathbb{P}(\theta_{n})$. Then, from Eq. \ref{condistri}, $\hat{\theta}_{n}|\theta_{0} \sim \mathcal{N}(\theta_{0}, \eta \mathbf{H}^{-1})$.
\end{proof}

\subsection{Proof of Proposition 2}
\label{app:pro2}
\begin{proposition}
Let $f(\theta_{n})$ be the probability density function of $\mathcal{N}(\theta_{0}, \eta \mathbf{H}^{-1})$. $\theta_{n, 1}, \cdots, \theta_{n, k}$ are i.i.d. samples drawn from $f(\theta_{n})$, $k$ is {\color{blue}the number of parameter sampling}. The inequality {\color{blue}$\mathbb{P}(\mathcal{D}(\mathcal{M}_{0}, \mathcal{M}_{n})\le \varepsilon) \geq 1-\alpha$} holds, if $\varepsilon$ satisfies that,
\begin{equation}\nonumber
\begin{aligned}
\mathbb{P}(\mathcal{D}(\mathcal{M}_{0}, \mathcal{M}_{n})\le \varepsilon)
&\approx \frac{1}{k}\sum_{i=1}^{k}\mathcal{I}[\mathcal{D}(\mathcal{M}_{0}; \theta_{n, i}) \le \varepsilon] \ge \frac{1 - \alpha}{1 - \beta} + \sqrt{\frac{\rm{log} (1-\beta)}{-2k}},
\label{eq:lemma1}
\end{aligned}
\end{equation}
where $\beta$ is a hyper-parameter ($0 <  \beta  \le \alpha\le 1$) and {\color{blue} $\mathcal{I}$} is the indicator function that returns 1 if its argument is true, and returns 0 otherwise.
\end{proposition}
%\textbf{Lemma 1}
%\emph{Let $f(\theta_{n})$ be the probability density function of $\mathcal{N}(\theta_{0}, \eta \mathbf{H}^{-1})$. $\theta_{n, 1}, \cdots, \theta_{n, k}$ is i.i.d. samples drawn from $f(\theta_{n})$.
%If $\varepsilon$ satisfies,
%\begin{equation}
%\begin{aligned}
%\mathbb{P}(\mathcal{D}(\mathcal{M}_{0}, \mathcal{M}_{n})\le \varepsilon)
%&\approx \frac{1}{k}\sum_{i=1}^{k}\mathds{1}[\mathcal{D}(\mathcal{M}_{0}; \theta_{n, i}) \le %\varepsilon] \ge \frac{1 - \alpha}{1 - \beta} + \sqrt{\frac{\rm{log} (1-\beta)}{-2k}}\\
%\text { then } & {\quad \mathbb{P}(\mathcal{D}(\mathcal{M}_{\star}, \mathcal{M}_{n})\le \varepsilon) %\geq 1-\alpha}
%%\label{eq:lemma1}
%\end{aligned}
%\end{equation}
%where $k$ is the number of parameter sampling times, and $\beta$ is a hyper-parameter ($0 < \alpha \le \beta \le 1$). $\mathds{1}$ is the indicator function that returns 1 if its argument is true, and returns 0 otherwise.
%}

\begin{proof}
By the Hoieffding's inequality,
\begin{equation}\nonumber
\mathbb{P}(b - a \ge \varepsilon_{1}) \le e^{-2k\varepsilon_{1}^{2}}
\end{equation}
\begin{align}\nonumber
\rm{where} \quad & a = \int \mathds{1}[\mathcal{D}(\mathcal{M}_{0}, \mathcal{M}_{n})\le \varepsilon]h(\theta_{n})d\theta_{n}\\
&b = \frac{1}{k}\sum_{i=1}^{k} \mathds{1}[\mathcal{D}(\mathcal{M}_{0}, \mathcal{M}_{n, i}) \le \varepsilon]. \nonumber
\end{align}
%Symmetrically, this inequality is also valid for another side of the difference
%\begin{equation}
%\mathbb{P} ( - a + b \ge \varepsilon_{1}) \ge 1 - e^{-2k\varepsilon_{1}^{2}}
%\end{equation}
%%By adding the two above inequalities, we can obtain two-sided variant of this inequality
%%\begin{equation}
%%\mathbb{P}( | a - b| \ge \varepsilon_{1}) \le 2 e^{-2k\varepsilon_{1}^{2}}
%%\end{equation}
Therefore, when
\begin{equation}\nonumber
    k \ge \frac{\rm{log}(1 - \beta)}{-2\varepsilon_{1}^{2}},
\end{equation}
we can acquire $1 - \beta$ confidence interval $[a + \varepsilon_{1}, \infty)$ for $b$.

Furthermore, in order to guarantee that $\mathbb{P}(\mathcal{D}(\mathcal{M}_{0}, \mathcal{M}_{n}) \le \varepsilon) \ge 1 - \alpha$, we will take conservative estimation, i.e., ensuring that
\begin{align}\nonumber
   \frac{1}{k}\sum_{i=1}^{k}\mathbf{1}[\mathcal{D}(\mathcal{M}_{0}, \mathcal{M}_{n, i}) \le \varepsilon] &\ge \frac{1 - \alpha}{1 - \beta} + \varepsilon_{1}\\\nonumber
   &\ge \frac{1 - \alpha}{1 - \beta} + \sqrt{\frac{\rm{log} (1 - \beta)}{-2k}}.
\end{align}
Therefore, we can finally have at least $(1 - \beta)\cdot \displaystyle{\frac{1 - \alpha}{1 - \beta}} = (1 - \alpha)$ confidence guaranteeing $\mathcal{D}(\mathcal{M}_{0}, \mathcal{M}_{n}) \le \varepsilon$.
\end{proof}

\subsection{Proof of Proposition 3}
\label{app:pro3}
\begin{proposition}
Let $f(\theta;\eta C)$ be the density function of the distribution in $\textbf{Theorem 1}$ where C is an arbitrary positive semidefinite matrix. And denote $B$ as the definition domain for $\theta$. Then the follow function
\begin{equation}\nonumber
    p(\eta) = \int_{B} f(\theta;\eta C) d\theta,
\end{equation}
is an decreasing function with respect to $\eta$, i.e., an increasing function with respect to $n$.
\end{proposition}
\begin{proof}
For arbitrary $\eta_{1} \le \eta_{2}$,
\begin{align*}
    p(\eta_{1}) = & \int_{B} \frac{1}{2\pi\sqrt{|\eta_{1}C|}}\exp({-\theta^{\top}(\eta_{1} C)^{-1}\theta}) d\theta\\
                = & \int_{\sqrt{\eta_{2}/\eta_{1}}B} \frac{1}{2\pi\sqrt{|\eta_{2}C|}}\exp({-\theta^{\top}(\eta_{2} C)^{-1}\theta}) d\theta\\
                \ge & \int_{B} \frac{1}{2\pi\sqrt{|\eta_{2}C|}}\exp({-\theta^{\top}(\eta_{2} C)^{-1}\theta})d\theta = p(\eta_{2}).
\end{align*}
Thus, $p(\eta)$ is an decreasing function with respect to $\eta$.
\end{proof}

\section{Appendix for Supporting Regression-based Imputation}
\label{sec:regression}

The regression-based parametric imputation is to construct at least one parametric prediction model for each incomplete feature.
Specifically, for the incomplete feature $f_j$, $\mathbf{X}_{:j}$ is used to collect the samples $\mathbf{x}_i$ from $\mathbf{X}$ that have observed values of feature $f_j$ (i.e., $m_{ij}$ is 1 in $\mathbf{M}$).
As a result, the prediction model $\mathcal{M}_j$ is trained on feature $f_j$, using the training dataset $\mathbf{X}_{:j}$.
The MS divergence imputation loss function for $\mathcal{M}_j$ can be defined as
\begin{equation}\nonumber
\begin{aligned}
    \label{eq: SDILoss}
      \mathcal{L}_s (\mathbf{X}_{:j}) = \frac{1}{2n_j}\mathcal{S}_{\mathbf{m}}(\bar{\mathbf{X}}_{:j}, \mathbf{X}_{:j}) = \frac{1}{2n_j} \big[2OT_{\lambda} (\hat{\nu}_{\bar{{x}}_{:j}}, \hat{\mu}_{{x}_{:j}}) - \big(OT_{\lambda} (\hat{\nu}_{\bar{{x}}_{:j}}, \hat{\mu}_{\bar{{x}}_{:j}}) + OT^{}_{\lambda} (\hat{\nu}_{{x}_{:j}}, \hat{\mu}_{{x}_{:j}})\big)\big],
\end{aligned}
\end{equation}
where $n_j$ is the sample size in $\mathbf{X}_{:j}$.
$\hat{\mu}_{{x}_{:j}} \overset{def}{=} \frac{1}{n_j}\sum_{i=1}^{n_j} \delta_{x_{ij}}$ and  $\hat{\nu}_{\bar{{x}}_{:j}} \overset{def}{=} \frac{1}{n_j}\sum_{i=1}^{n_j} \delta_{\bar{x}_{ij}}$ denote the empirical measures over the original matrix $\mathbf{X}_{:j}$ and the predicted matrix $\bar{\mathbf{X}}_{:j}$, respectively.
The optimal transport metric $OT_{\lambda} (\hat{\nu}_{\bar{{x}}_{:j}}, \hat{\mu}_{{x}_{:j}})$ over $\hat{\nu}_{\bar{{x}}_{:j}}$ and $\hat{\mu}_{{x}_{:j}}$ can be defined as
\begin{equation}\nonumber
\begin{aligned}
      OT_{\lambda} (\hat{\nu}_{\bar{{x}}_{:j}}, \hat{\mu}_{{x}_{:j}}) = \min_{\mathbf{P} \in \Gamma_{n_{j}, n_{j}}} \langle \mathbf{P} , \mathbf{C}\rangle + \lambda H(\mathbf{P}).
\label{eq:A-regu}
\end{aligned}
\end{equation}
The cost matrix $\mathbf{C} : = \{f_c(\bar{{x}}_{i}, {x}_{j})\}_{ij} \in \mathbb{R}^{n_{j}\times n_{j}}$, where $f_c({x}, {y}) = |{x} - {y}|$ is the cost function.
Besides
$\langle \mathbf{P}, \mathbf{C}\rangle = {\rm tr}(\mathbf{P}^{\top}\mathbf{C})$ is the Frobunius dot-product of the $\mathbf{P}$ and $\mathbf{C}$ matrices.
$H(\mathbf{P})$ is the entropy of the transport plan matrix $\mathbf{P}$.

\section{Appendix for  Additional Experimental Results}
\label{sec:appendix-results}

\subsection{Implementation Details}
\label{sec:appendix-setting}

\textbf{Implementation details.}
For all regression-based imputation methods, the learning rate is set to 0.3, and the number of iterations is set to 100.
In particular, the number of decision trees in MissFI is set to 6.
The imputation times in MICE are 20.
For all reconstruction-based imputation methods, the learning rate is 0.001, the dropout rate is 0.5, the training epoch is 30, and the batch size is 128.
The ADAM algorithm is utilized to train networks.
MIDAE is a 2-layer with 128 units per layer network.
For VAEI, the encoder and decoder are fully connected networks with two hidden layers, each with 20 neurons per layer, and the latent space was 10-dimensional.
HIVAE uses only one dense layer for all the parameters of the encoder and decoder, each with 10 neurons per layer.
In GINN, the discriminator used is a simple 3-layer feed-forward network trained 5 times for each optimization step of the generator.
In GAIN, both generator and discriminator are modeled as 2-layer fully connected network.

\begin{table}[t]\small
\centering
\caption{Post-imputation evaluation (i.e., AUC and MAE) over four real-world datasets}
\label{Tab:Post-imputation}
\setlength{\tabcolsep}{7.5pt}
\begin{tabular}{|c|c|c|c|c|c|}
\hline
Metric&Dataset& HIVAE& \textsf{SCIS}-HIVAE& GAIN& \textsf{SCIS}-GAIN\\ \hline
\multirow{2}{*}{AUC} &\emph{Trial} &92.43 ($\pm$ 3.40)&\textbf{92.55 ($\pm$2.31)}&90.25 ($\pm$ 3.98)&90.40 ($\pm$4.01)\\\cline{2-6}
&\emph{Surveil} &\textbf{96.89 ($\pm$ 1.20)}& 96.70 ($\pm$ 0.89)&94.90 ($\pm$2.01)&95.01 ($\pm$ 2,53)\\\hline
\multirow{2}{*}{MAE} &\emph{Weather} &98.22 ($\pm$ 8.61)&\textbf{97.25 ($\pm$ 9.24)}&100.26 ($\pm$7.83)&99.89 ($\pm$9.22)\\\cline{2-6}
&\emph{Search} &$-$&\textbf{82.20($\pm$ 6.02)}&89.14 ($\pm$ 9.54)& 89.14 ($\pm$ 9.90)\\\hline
\end{tabular}
\end{table}

\subsection{Post-imputation Prediction}
The ultimate goal of imputing missing data is to benefit the \emph{downstream data analytics}, e.g., regression and classification.
In the last set of experiments, we verify the superiority of \textsf{SCIS} over the original parametric imputation methods on \emph{post-imputation prediction} task.

%{\color{blue}The regression task is to predict the count of new cases confirmed after a positive test.}
The post-imputation prediction results are depicted in Table \ref{Tab:Post-imputation}, with the classification task over \emph{Weather} and \emph{Search} and the regression task over \emph{Trial} and \emph{Surveil}.
The larger AUC value corresponds to the better post-imputation prediction effect, while RMSE is opposite.
In particular, the imputation methods are first employed to impute missing values in the input incomplete datasets.
Then, a regression/classification model is trained with three fully connected layers over the imputed data.
The training epoch is 30, the learning rate is 0.005, and the dropout rate is 0.5.

The post-imputation prediction results are depicted in Table~\ref{Tab:Post-imputation}. The larger AUC value corresponds to the better prediction effect, while RMSE is opposite.
We can observe that, the prediction performance under different imputation algorithms is consistent with the imputation performance of these algorithms, i.e., the \textsf{SCIS} ones have approximate accuracy with original ones.
%{\color{blue}In particular, \textsf{SCIS} exceeds the corresponding original method by \% in average, and it increases up to \% for .}
